# Supplementary material for: Transformer-based Entity Legal Form Classification
Source: arXiv:2310.12766 source file (2023-10-19)
Supplement: Supplementary file 1 [file 05_appendix.tex]

\appendix

\begin{table}
\resizebox{\textwidth}{!}{\begin{tabular}{lr|rr|rr|rr|rr|rr}

\multicolumn{12}{l}{\textbf{Traditional model evaluation: abbreviations and preprocessing}} \\
\midrule
{} & &  \multicolumn{2}{c}{\textbf{CNB}} &  \multicolumn{2}{c}{\textbf{CNB + lowercase}} & \multicolumn{2}{c}{\textbf{CNB + prep}} & \multicolumn{2}{c}{\textbf{CNB + abbr}} & \multicolumn{2}{c}{\textbf{CNB + prep + abbr}} \\
{} &  num\_samples &  F1 &  F1-macro &  F1 &  F1-macro  &  F1 &  F1-macro &  F1 &  F1-macro &  F1 &  F1-macro \\
\midrule
DE    &       135079 &    0.8947 &    0.5022 &         0.8940 &         0.4988 &           0.9201 &           0.5275 &           0.9142 &           0.5332 &  \textbf{0.9431} &  \textbf{0.5595} \\
IT    &       104968 &    0.8657 & \textbf{0.2328} &   0.8656 &         0.2271 &  \textbf{0.8660} &           0.2253 &           0.8657 &  0.2328 &  0.8660 &           0.2253 \\
NL    &        89748 &    0.9621 &    0.6366 &         0.9622 &         0.6378 &           0.9629 &           0.6306 &           0.9621 &  \textbf{0.6426} &  \textbf{0.9630} &           0.6367 \\
ES    &        84231 &    0.9348 &    0.4728 &         0.9350 &         0.4680 &  \textbf{0.9429} &           0.4775 &           0.9349 &           0.4772 &          0.9429 &           0.4883 \\
GB    &        74847 &  \textbf{0.9424} & 0.2670 &     0.9419 &         0.2673 &  0.9424 &  \textbf{0.2687} &  0.9424 &           0.2670 &  0.9424 &  0.2687 \\
FR    &        59973 &    0.4390 &    0.1555 &         0.4388 &         0.1540 &  \textbf{0.4408} &           0.1541 &           0.4391 &  \textbf{0.1562} &  0.4408 &           0.1545 \\
DK    &        56226 &  \textbf{0.9160} & \textbf{0.5173} &         0.9145 &         0.5050 &           0.9068 &           0.4334 &           0.9160 &           0.5173 &           0.9068 &           0.4334 \\
US-DE &        54156 &    \textbf{0.9653} &    \textbf{0.4540} &         0.9621 &         0.4482 &           0.9593 &           0.4505 &           0.9653 &           0.4540 &           0.9593 &           0.4505 \\
SE    &        48083 &    0.9714 &    0.4838 &         0.9715 &         0.4839 &           \textbf{0.9721} &           \textbf{0.4858} &           0.9714 &           0.4840 &           0.9721 &           0.4858 \\
FI    &        35587 &    0.9797 &    0.5039 &         \textbf{0.9799} &         0.4982 &           0.9797 &           0.4973 &           0.9797 &           \textbf{0.5096} &           0.9797 &           0.5031 \\
LU    &        33683 &    \textbf{0.8227} &    \textbf{0.3814} &         0.8203 &         0.3841 &           0.7455 &           0.3694 &           0.8227 &           0.3823 &           0.7455 &           0.3703 \\
NO    &        32996 &    0.9848 &    0.5864 &         \textbf{0.9853} &         0.5909 &           0.9853 &           \textbf{0.6048} &           0.9848 &           0.5865 &           0.9853 &           0.6048 \\
AT    &        24433 &    0.8963 &    0.5113 &         0.8978 &         0.5040 &           0.9162 &           0.5021 &           0.9069 &           0.5192 &           \textbf{0.9269} &           \textbf{0.5223} \\
BE    &        23969 &    0.3495 &    0.1171 &         0.3622 &         \textbf{0.1214} &           0.3719 &           0.1141 &           0.3495 &           0.1202 &           \textbf{0.3720} &           0.1172 \\
KY    &        20541 &    0.6590 &    0.3565 &         \textbf{0.6671} &         \textbf{0.3583} &           0.6584 &           0.3556 &           0.6589 &           0.3564 &           0.6583 &           0.3556 \\
PL    &        20173 &    0.9393 &    0.4277 &         0.9662 &         0.4649 &           \textbf{0.9689} &           0.4629 &           0.9393 &           0.4324 &           0.9689 &           \textbf{0.4659} \\
AU    &        15350 &    0.8298 &    0.2638 &         \textbf{0.8337} &         \textbf{0.2921} &           0.8197 &           0.2305 &           0.8298 &           0.2638 &           0.8197 &           0.2305 \\
IE    &        15294 &    \textbf{0.8611} &    0.4411 &         0.8535 &         0.4276 &           0.8552 &           0.4282 &           0.8611 &           \textbf{0.4445} &           0.8554 &           0.4404 \\
VG    &        15086 &    0.7784 &    0.1815 &         \textbf{0.8550} &         \textbf{0.1833} &           0.8532 &           0.1691 &           0.7785 &           0.1815 &           0.8532 &           0.1689 \\
CZ    &        14477 &    0.9800 &    0.4301 &         0.9814 &         \textbf{0.4371} &           \textbf{0.9829} &           0.4307 &           0.9800 &           0.4301 &           0.9829 &           0.4307 \\
EE    &        13824 &    0.9941 &    0.5672 &         0.9949 &         0.5887 &           0.9949 &           0.5907 &           0.9942 &           0.5765 &           \textbf{0.9950} &           \textbf{0.6000} \\
CH    &        13742 &    0.8890 &    0.3073 &         0.8871 &         \textbf{0.3227} &           \textbf{0.8989} &           0.3186 &           0.8865 &           0.3070 &           0.8967 &           0.3178 \\
HU    &        10041 &    0.9155 &    \textbf{0.4921} &         \textbf{0.9176} &         0.4917 &           0.9163 &           0.4890 &           0.9156 &           0.4921 &           0.9163 &           0.4890 \\
JP    &         9690 &    0.1089 &    0.1508 &         0.1097 &         0.1523 &           \textbf{0.2746} &           \textbf{0.1832} &           0.1089 &           0.1508 &           0.2746 &           0.1832 \\
LI    &         9458 &    0.9389 &    0.7569 &         0.9414 &         0.7602 &           \textbf{0.9522} &           \textbf{0.7708} &           0.9389 &           0.7573 &           0.9521 &           0.7676 \\
US-CA &         6176 &    0.9234 &    \textbf{0.3741} &         \textbf{0.9252} &         0.3697 &           0.9244 &           0.3536 &           0.9234 &           0.3741 &           0.9244 &           0.3536 \\
US-NY &         4836 &    \textbf{0.9353} &    \textbf{0.4835} &         0.9332 &         0.4704 &           0.9344 &           0.4771 &           0.9353 &           0.4835 &           0.9340 &           0.4763 \\
MX    &         3184 &    \textbf{0.8470} &    \textbf{0.2978} &         0.8417 &         0.2899 &           0.8411 &           0.2843 &           0.8467 &           0.2976 &           0.8411 &           0.2847 \\
PA    &         2925 &    0.8769 &    \textbf{0.3558} &         0.8769 &         0.3523 &           \textbf{0.8783} &           0.3552 &           0.8769 &           0.3558 &           0.8783 &           0.3553 \\
BG    &         2335 &    0.4655 &    0.2911 &         \textbf{0.4874} &         \textbf{0.2992} &           0.4385 &           0.2205 &           0.4655 &           0.2911 &           0.4385 &           0.2205 \\
\bottomrule
\end{tabular}}
\end{table}
